# Supplementary material for: Uncertainty in Extreme Multi-label Classification
Source: arXiv:2210.10160 source file (2022-10-18)
Supplement: Supplementary file 1 [file expsettings.tex]

\section{Detailed Experimental Settings}
\label{appendix:expsettings}

In this section, we describe the details of our experimental settings.

\subsection{Experimental Datasets}
\label{appendix:datasets}

Table~\ref{table:datasets} represents the detailed statistics of six large-scale real-world XMC datasets~\cite{you2019attentionxml} in our experiments.
Note that these six publicly available benchmark datasets are publicly available at \url{https://github.com/yourh/AttentionXML}.
The sparse representations for \xrlinear and training/testing data splits are also consistent with previous studies~\cite{you2019attentionxml,chang2020xmctransformer,zhang2021fast,jiang2021lightxml}.

\begin{table}[!h]
\centering
\caption{The statistics of six experimental datsets. Note that $n_{\text{train}}, n_{\text{test}}$ are the numbers of training and testing instnaces. 
        $\abs{\cD_{\text{train}}}$ and $\abs{\cD_{\text{test}}}$ refer to the number of word tokens in the training and test corpus, respectively.
        $d$ is the dimension of \tfidf feature vector.
        $L$ is the number of labels while $\bar{L}$ the average number of labels per instance.
        $\bar{n}$ the average number of instances per label.
}
\label{table:datasets}
%\resizebox{1.0\textwidth}{!}{
    \begin{tabular}{c|rrrrrrrr}
    \toprule
        Dataset            & $n_{\text{train}}$ & $n_{\text{test}}$ & $\abs{\cD_{\text{train}}}$ &  $\abs{\cD_{\text{test}}}$ & $d$       & $L$       & $\bar{L}$ & $\bar{n}$ \\
        \midrule
        \eurlex         &       15,449    &           3,865  &              19,166,707  &                 4,741,799 &   186,104 &     3,956 &     5.30  &     20.79 \\
        \wikis          &       14,146    &           6,616  &              29,603,208  &                13,513,133 &   101,938 &    30,938 &    18.64  &      8.52 \\
        \amzsmall       &      490,449    &         153,025  &             119,981,978  &                36,509,660 &   135,909 &   670,091 &     5.45  &      3.99 \\
        \amzcat         &    1,186,239    &         306,782  &             250,940,894  &                64,755,034 &   203,882 &    13,330 &     5.04  &    448.57 \\
        \wikil          &    1,779,881    &         769,421  &           1,463,197,965  &               632,463,513 & 2,381,304 &   501,070 &     4.75  &     16.86 \\
        \amzlarge       &    1,717,899    &         742,507  &             174,559,559  &                75,506,184 &   337,067 & 2,812,281 &    36.04  &     22.02 \\
        \bottomrule
        \end{tabular}
%}
\end{table}

\subsection{Evaluation Tasks and Evaluation Metrics}
\label{appendix:tasks}

To evaluate the quality of uncertainty quantification, we consider three different evaluation tasks, including (1) predictive performance, (2) misclassification detection, and (3) out-of-distribution (OOD) deteciton.

\mysection{Task 1: Predictive Performance}
The prediction accuracy should not be sacrificed while modeling uncertainty.
Actually, appropriately modeling uncertainty usually can lead to improvements on predictive accuracy~\cite{gal2016dropout, Gal2016Uncertainty,malinin2020uncertainty,malinin2019uncertainty}.
For the task of predictive performance, we follow conventional research~\cite{yu2020pecos,chang2020xmctransformer,zhang2021fast,jiang2021lightxml,you2019attentionxml,prabhu2018parabel,khandagale2020bonsai} on XMC to evaluate top-ranked labels with conventional ranking evaluation metrics Precision@$k$ (P@$k$) and Recall@$k$ (R@$k$), where $k=\{1,3,5\}$ consists of high-ranked positions.
The two metrics are defined as:
\begin{equation*}
    \text{P@}k=\frac{1}{k} \sum_{i=1}^k y_{\text{rank}(i)}; \text{R@}k=\frac{1}{\sum_{\ell\in \cL} y_{\ell}} \sum_{i=1}^k y_{\text{rank}(i)},
\end{equation*}
where $y_{\ell}=\{0, 1\}$ represents if the instance has the label $\ell$; $\text{rank}(i)$ represents the rank-$i$ label.

\mysection{Task 2: Misclassification Detection}
Suppose we have an oracle to know the number of true labels $r$ for the testing instance $\bx$.
The top-$r$ ranked labels can artifically be treated as positive classification while the remaining ones are negative.
We evaluate the label-level uncertainty with the task of misclassification detection, which is usually considered for evaluating classification uncertainty~\cite{shelmanov2021certain}.
In particular, given a testing instance $\bx$, higher uncertainty for a label would lead to higher odds to be \emph{misclassified} (i.e., ranked in incorrect range).
The task can be assessed via area under the ROC curve (AUROC)~\cite{hendrycks2016baseline} for each testing instance and its label rankings.

\mysection{Task 3: Out-of-Distribution (OOD) Detection}
OOD detection is one of the popular tasks for evaluating instance-level uncertainty~\cite{malinin2020uncertainty,charpentier2020posterior}.
Precisely, predictions of a model would have higher uncertainty for testing instances that are out of the training distribution.
In our experiments, we first train XMC models with the training data of one of the six datasets, and then mix its testing data with one of the other five datasets as OOD instances.
AUROC~\cite{hendrycks2016baseline} is also considered as the evaluation metric for this task.

%Note that we evaluate all three approaches of generating XMC model ensembles (i.e., \emph{Bagging}, \emph{Boosting}, and \emph{Boosted Bagging}) described in Section~\ref{section:method:generation} for all tasks.
%For evaluating uncertainty quality, we examine three methods mentioned in Section~\ref{section:prelim:ensemble}, including \emph{probability variance}~(PV), \emph{total uncertainty}~(TU), and \emph{knowledge uncertainty}~(KU), to derive uncertainty measurements.

\subsection{Experimental Details and Hyper-parameter Settings}
 
Experiments described in Sections~\ref{section:exp:task1}, \ref{section:exp:task2}, \ref{section:exp:task3}, and \ref{section:exp:efficiency} without a need of GPUs are conducted on an AWS {\sf x1.32xlarge} instance with 128 CPU cores based on four Intel Xeon E7-8880 v3 \@ 2.30GHz processors and 1,952 GiB memory.
Experiments described in Section~\ref{section:exp:deep} with needs of GPUs are conducted on an AWS {\sf p3dn.24xlarge} instance with 96 CPU cores based on four Intel Xeon Platinum 8175M \@2.50GHz processors, 96 GiB memory, and 8 NVIDIA V100 Tensor Core GPUs with 32 GB of memory each.

For XR-Linear as our base XMC model, we establish hierarchical label trees based on Positive Instance Feature Aggregation (PIFA)~\cite{yu2020pecos} and 8-means (i.e., $B_t = 8$).
After training, model weights smaller than $1e-3$ are ignored for reducing disk space consumption, following the settings of \xrlinear~\cite{yu2020pecos}.
For inference, the beam size $b$ and the number of top-ranked labels $k$ in beam search are set as 50 and 100.
For the \emph{Bagging} ensemble approach, we bootstrap datasets with the identical size to the training dataset for training individual models.
For the \emph{Boosting} ensemble approach, we set the hyper-parameter $\alpha=0.5$.
For all ensemble-based approaches in the experiments (i.e., all methods except the single model), the number of model ensembles $M$ is 10 for ensemble generation.
In addition, training an enormous ensemble for XMC models is unrealistic due to both time and space constraints.
For instance, a single \xrlinear model for the {\sf Amazon-3M} dataset would take more than 100 GB in the disk space and could require days to train.
For \xrtransformer as our base XMC model, we follow the instructions in the original paper and adopt hyper-parameters described in \url{https://github.com/amzn/pecos/tree/mainline/examples/xr-transformer-neurips21/params} to train every individual \xrtransformer model.
All deep learning models using transformers use the {\sf bert-base-uncased} model as the pretrained model~\cite{devlin2018bert}.
