# Supplementary material for: Uncertainty in Extreme Multi-label Classification
Source: arXiv:2210.10160 source file (2022-10-18)
Supplement: Supplementary file 2 [file instunc.tex]

\section{Explainability of Instance-level Uncertainty}
\label{appendix:instunc}

Here we present the explainability of instance-level total uncertainty discussed in Section~\ref{section:method:uncertainty} with more details. First, we let $Z_\ell = p(\bx\mid y_\ell) / p(y_\ell\mid \bx)$ is the normalized density for each label $l\in \cL$.

\begin{align*}
 \sum_{\ell\in \cL} \cH[p(y_\ell)] & = \sum_{\ell\in \cL} - \ln p(y_\ell\mid \bx) \\ 
      \text{(Apply $Z_\ell$ to obtain joint likelihood)}
    & = -\sum_{\ell\in \cL} \ln p(y_\ell\mid \bx) \frac{Z_\ell}{Z_\ell} = -\sum_{\ell\in \cL} \ln \frac{p(\bx\mid y_\ell)}{Z_\ell} \\
    &  = -\sum_{\ell\in \cL} \ln p(\bx\mid y_\ell) - \sum_{\ell\in \cL} Z_\ell \\
      \text{(Apply Bayes rule)}
    & = -\sum_{\ell\in \cL} \ln \frac{p(y_\ell\mid \bx)p(\bx)}{p(y_\ell)} - \sum_{\ell\in \cL} Z_\ell \\
    & = -\ln \prod_{\ell\in \cL} \frac{p(y_\ell\mid \bx)p(\bx)}{p(y_\ell)} - \sum_{\ell\in \cL} Z_\ell\\
    & = -\ln \prod_{\ell\in \cL} p(y_\ell\mid \bx)- L \ln p(\bx) + \ln \prod_{\ell\in \cL} p(y_\ell) - \sum_{\ell\in \cL} Z_\ell \\
    \text{(Assume conditional independence of $y_\ell$)} 
    & =  -\ln p(y_1, \dots, y_L\mid \bx)  - L \ln p(\bx) + \ln \prod_{\ell\in \cL} p(y_\ell) - \sum_{\ell\in \cL} Z_\ell \\
    \text{(Apply Bayes rule)}
    & = -\ln \frac{p(\bx \mid y_1, \dots, y_L) \prod_{\ell\in \cL} p(y_\ell)}{p(\bx)} - L \ln p(\bx)  + \ln \prod_{\ell\in \cL} p(y_\ell) - \sum_{\ell\in \cL} Z_\ell \\
    & = \underbrace{-\ln p(\bx\mid y_1, \dots y_L)}_{\text{Knowledge Uncertainty}} \underbrace{-(L-1)\ln p(\bx)}_{\text{Data Uncertainty}} - \sum_{\ell\in \cL} Z_\ell.
\end{align*}
